# Supplementary material for: Contrastive Meta Learning with Behavior Multiplicity for Recommendation
Source: arXiv:2202.08523 source file (2022-02-17)
Supplement: Supplementary file 1 [file appendix.tex]

\section{Appendix}
\label{sec:appendix}
